# Supplementary material for: Unstructured un-split geometrical Volume-of-Fluid methods -- A review
Source: arXiv:2007.02860 source file (2020-07-06)
Supplement: Supplementary file 1 [file appendix.tex]

\section{Mesh addressing complexity}
\label{sec:appa}

To iterate over all points of all faces of a cell, in order to perform an intersection between each face and a half-space, incurs a substantial number of iterations, compared to the direct face-point access on structured meshes. On a structured mesh each cell center is defined with an index triplet $(i, j, k)$. Accessing a cell face requires adding $\pm\frac{1}{2}$ to a corresponding index of the cell triplet. Directly addressing face centers of the $i+\frac{1}{2}$ faces by changing their $y$ coordinate results in simply increasing the third index of the face triple: $(i+\frac{1}{2},j, k+l)$. This operation has a constant complexity per face of $\Oh_f= 1$. 

On an unstructured mesh, a search operation must be performed on a per-cell basis to find the face in a specific direction. The search algorithms used to locate a face in a specific direction rely on the connections between mesh elements. Using a search algorithm that relies on edge-face connectivity information would result in a worst-case complexity per face of $\Oh_f= N_{f,e}$ where $N_{f,e}$ is the number of faces that share an edge $e$ with a face $f$. This number is not large: for hexahedral cells $N_{e,f} = 12$. However, that number becomes a large constant factor that multiplies the overall complexity of an algorithm that loops over all mesh faces $\Oh = N_f \Oh_f = 12 N_f$, where $N_f$ is the number of all faces in the mesh. Therefore, an algorithm that requires \emph{directional access} to a specific face has a $12$ times greater access complexity on an unstructured than on a structured mesh, even if both meshes are composed of cubical cells. Moreover, because the unstructured mesh elements are not sequentially addressed from memory, cache-based memory access optimizations \citep[sec. 9.9]{Fog2015} are difficult to implement. A re-ordering of unstructured addressing information based on direction conditions can be performed once, if the mesh is not changed topologically. However, the main advantage of unstructured meshes is their ability to support local and dynamic \ac{AMR}, that would require the re-ordering to be executed after each topological change.
